# Supplementary material for: Searching for modular companions
Source: arXiv:1902.05199 ancillary file (2019-02-14)
Supplement: Supplementary file 1 [file ModularCompanionsProgram.pdf]

Required packages:

```
> with(LinearAlgebra) :
```

We use a precision of 50 digits for floating point calculations.

```
> Digits:=50;
```

```
Digits := 50
```

(1)

Rogers dilogarithm function:

```
> L:=proc(x) :  
  if x=0 then: return 0; fi:  
  if x=1 then: return Pi^2/6; fi:  
  return dilog(1-x) + log(x)*log(1-x)/2;  
end:
```

ser(f,t,var)

Given a function `f` in variable `var`, find its Taylor series at var=0 up to `var^t` terms.

Try:

```
ser(1/(1-q),10,q);
```

```
> ser:=proc(f,t,var) :  
  return(convert(series(f,var=0,t+1),polynom)) :  
end:
```

serexp(f,t:=6,var:=epsilon)

Given a function `f` in variable `var`, find the Taylor series of  $1 + f + (f^2/2!) + \dots + (f^t/t!)$  at var=0 up to `var^t` terms.

Default value of `t` is 6 and that of `var` is epsilon.

Try:

```
serexp(q+q^2,3,q);
```

```
> serexp:=proc(f,t:=6,var:=epsilon)  
  local ans:=1,i,temp:=1;  
  for i from 1 to t do:  
    temp:=ser(temp*f,t,var) :  
    ans:=ans+ temp/factorial(i) :  
  end:  
end:
```

findC(L)

Given a list  $L = (L[1], L[2], \dots, L[n])$ , consider the periodic product  $P = (1-q)^{L[1]} * (1-q^2)^{L[2]} * \dots * (1-q^n)^{L[n]} * (1-q^{(n+1)})^{L[1]} \dots$

Finds a constant  $C$  such that  $q^C * P$  is modular.

Try (to find  $C$  corresponding to first Rogers-Ramanujan identity):

```
findC([-1,0,0,-1,0]);
```

```

> findC:=proc(L)
  local i, m, ans:=0:
  m:=nops(L):
  for i from 1 to m-1 do:
    ans:=ans+L[i]*m/24 - i*(m-i)*L[i]/4/m;
  end:
end:

```

```
ppoly(p,var:=X)
```

Define a sequence of polynomials in variable `var` (default=X)

for  $p=1,2,\dots$

such that:

$ppoly(1,X)=X$ ,

$ppoly(p+1, X) = (X^2 + X) * d(ppoly(p,X))/dX$

We have that:

$Li_{\{2-r\}}(Q) = ppoly(r-1,Q/(1-Q))$  for  $r \geq 1$ .

Try:

```
ppoly(1,X);
```

```
subs(X=Q/(1-Q), ppoly(1,X));
```

```
ppoly(2,X);
```

```
subs(X=Q/(1-Q), ppoly(2,X));
```

```

> ppoly:=proc(p, var:=X) :
  if p=1 then: return var: fi:
  return diff(ppoly(p-1, var), var) * (var^2+var) :
end:

```

```
exparg(B,xi,T,J:=1,cutoff:=4,var:=epsilon)
```

This is the argument of exponential in equation (12) of the paper.

$B = B_i$ ,

$xi = xi_i$ ,

$T = t_i$ ,

$J = J_i$ ,

cutoff = we take the summation over `p` up to  $p=cutoff$ . Default is 4.

var = this is actually the  $\sqrt{\epsilon}$  from the paper. so, the epsilon here is the  $\sqrt{\epsilon}$  from the paper.

```

> exparg:=proc(B,xi,T,J:=1,cutoff:=4,var:=epsilon)
  local p:
  return (B + xi/2)*T*var
    - add(
      J^(p-1)
      *expand(bernoulli(p,T/var)*var^(2*p-2))
      *subs(X=xi/J,ppoly(p-1,X))/factorial(p)
      , p=3..cutoff):
end:

```

```
int2all(f,Atinv,cutoff:=30,var1:=t1,var2:=t2)
```

consider a function `f` in variables var1 and var2. (Default t1, t2, respectively.)

consider a matrix  $A_t$  (which is  $A$ -tilde from equations (9) and (14)) whose inverse is  $A_{tinverse}$

calculates the value from equation (14) with  $C_{2p}$  replaced by  $f$ .

we cutoff  $f$  by expanding it up to terms  $\text{var1}^{\text{cutoff}} * \text{var2}^{\text{cutoff}}$ .

```
> int2all:=proc(f,Atinv,cutoff:=30,var1:=t1,var2:=t2)
  option remember:
  local xv,ip,ex,g,i,j,ans:=0,x1,x2:
  xv:=Matrix(2,1,[x1,x2]);
  ip:=((Transpose(xv).Atinv.xv)[1][1])/2;
  ex:=expand(ser(ser(exp(ip),cutoff+1,x1),cutoff+1,x2));
  g:=ser(ser(f,cutoff+1,var1),cutoff+1,var2):
  for i from 0 to cutoff do:
  for j from 0 to cutoff do:
    ans:=ans+coeff(coeff(g,var1,i),var2,j)
      *factorial(i)*factorial(j)*coeff(coeff(ex,x1,i),x2,
j):
  od:
  od:
  return ans:
end:
```

We now look at the Capparelli identities

```
> CapA:=Matrix(2,2,[4,6,6,12]);
Capxi1:=3;
Capxi2:=24;
CapAt:=CapA+DiagonalMatrix([Capxi1,Capxi2]);
CapAtinv:=MatrixInverse(CapAt);
```

$$CapA := \begin{bmatrix} 4 & 6 \\ 6 & 12 \end{bmatrix}$$

$$Capxi1 := 3$$

$$Capxi2 := 24$$

$$CapAt := \begin{bmatrix} 7 & 6 \\ 6 & 36 \end{bmatrix}$$

$$CapAtinv := \begin{bmatrix} \frac{1}{6} & -\frac{1}{36} \\ -\frac{1}{36} & \frac{7}{216} \end{bmatrix} \quad (2)$$

expargcutoff is the cutoff on the values of p in equation (12)  
 expcutoff is cutoff for the exponential function in equation (12)

```
> expargcutoff:=10;
expcutoff:=expargcutoff-2;
expargcutoff:=10
expcutoff:=8
```

(3)

Now we multiply the exponentials in equation (12) for i=1 and i=2 to get the C\_p polynomials in equation (13)

Note that the epsilon here is sqrt(epsilon) from the paper.

Capwanted calculates the integrals (14) for all polynomials C\_p. The terms corresponding to odd values of p are 0

and the ones corresponding to even values are the ones that lead to constants c\_p in (14).

```
> Capexptwovar:=serexp(ser(exparg(B1,Capxi1,T1,1,expargcutoff)+
exparg(B2,Capxi2,T2,3,expargcutoff),expcutoff,epsilon),
expargcutoff):
Capwanted:=ser(int2all(Capexptwovar,CapAtinv,30,T1,T2),
expargcutoff,epsilon):
```

Capc1 is the constant c1 from equation (14).

Similarly, Capc2 is c2, Capc3 is c3, Capc4 is c4.

Note again that epsilon here is the sqrt(epsilon) from the paper.

```
> Capc1:=coeff(Capwanted,epsilon,2):
Capc2:=coeff(Capwanted,epsilon,4):
```

```
Capc3:=coeff(Capwanted,epsilon,6):
Capc4:=coeff(Capwanted,epsilon,8):
```

The gamma value is stored in Capg

```
> Capg:=simplify(C + (2*Capxi1+1)/24 + (2*Capxi2+3)/24);
```

$$Capg := C + \frac{29}{12}$$

(4)

The expressions on the right-hand sides of (17) - (19) are stored below.

```
> Capexpr1:=simplify(Capc1 - Capg):
Capexpr2:=simplify(Capc2 - Capg*Capc1 + Capg^2/2):
Capexpr3:=simplify(Capc3 - Capg*Capc2 + Capg^2/2*Capc1 -
Capg^3/6):
Capexpr4:=simplify(Capc4 - Capg*Capc3 + Capg^2/2*Capc2 -
Capg^3/6*Capc1 + Capg^4/24):
```

Let us check that the constraints are all equal to 0 for the first Capparelli identity

```
> CapC:=findC([0,-1,-1,0,0,0,0,0,-1,-1,0,0]);
subs(C=CapC,B1=0,B2=0,Capexpr1);
subs(C=CapC,B1=0,B2=0,Capexpr2);
subs(C=CapC,B1=0,B2=0,Capexpr3);
subs(C=CapC,B1=0,B2=0,Capexpr4);
```

$$CapC := -\frac{1}{24}$$

0  
0  
0  
0

(5)

Now we consider general B1 and B2. We solve equation (16) for C and substitute this into (17) - (19).

```
> CapCval:=simplify(solve(Capexpr1=0,C));
Capeq1:=expand(simplify(subs(C=CapCval,Capexpr2)));
Capeq2:=expand(simplify(subs(C=CapCval,Capexpr3)));
Capeq3:=expand(simplify(subs(C=CapCval,Capexpr4)));
```

$$CapCval := -\frac{1}{24} + \frac{1}{24} B1 + \frac{1}{12} B1^2 + \frac{7}{432} B2^2 + \frac{5}{144} B2 - \frac{1}{36} B2 B1$$

$$Capeq1 := -\frac{1}{288} B1^2 B2 + \frac{5}{576} B1 B2^2 - \frac{7}{576} B1^2 - \frac{199}{20736} B2^2 + \frac{49}{1728} B2 B1$$

$$- \frac{1}{144} B1^3 - \frac{113}{31104} B2^3 + \frac{1}{1152} B1 + \frac{149}{6912} B2$$

$$Capeq2 := -\frac{31}{31104} B1^2 B2^2 + \frac{31}{10368} B1^2 B2 - \frac{127}{62208} B1 B2^2 - \frac{173}{279936} B1 B2^3$$

$$+ \frac{19}{7776} B2 B1^3 - \frac{37}{20736} B1^2 - \frac{5641}{746496} B2^2 + \frac{1093}{62208} B2 B1 + \frac{2105}{6718464} B2^4$$

$$\begin{aligned}
& -\frac{7}{5184} B1^3 - \frac{7}{5184} B1^4 + \frac{79}{1119744} B2^3 + \frac{31}{6912} B1 + \frac{335}{41472} B2 \\
\text{Capeq3} := & \frac{71}{165888} B1^4 B2 - \frac{721}{497664} B1^3 B2^2 + \frac{1373}{995328} B1^2 B2^3 - \frac{565}{17915904} B1 B2^5 \\
& - \frac{20657}{35831808} B1 B2^4 + \frac{2161}{442368} B1^2 B2^2 + \frac{5329}{1327104} B1^2 B2 - \frac{19171}{7962624} B1 B2^2 \\
& - \frac{32849}{11943936} B1 B2^3 - \frac{1465}{331776} B2 B1^3 - \frac{3157}{884736} B1^2 - \frac{262765}{31850496} B2^2 \\
& + \frac{55687}{2654208} B2 B1 + \frac{160699}{286654464} B2^4 - \frac{523}{663552} B1^3 + \frac{299}{221184} B1^4 \\
& + \frac{793}{143327232} B2^3 + \frac{1}{41472} B1^6 + \frac{1}{9216} B1^5 + \frac{100903}{1074954240} B2^5 + \frac{12769}{1934917632} B2^6 \\
& + \frac{161}{49152} B1 + \frac{11393}{1474560} B2 + \frac{1}{41472} B1^5 B2 - \frac{1}{18432} B1^4 B2^2 - \frac{11}{2239488} B1^3 B2^3 \\
& + \frac{901}{17915904} B1^2 B2^4
\end{aligned} \tag{6}$$

We now solve these equations simultaneously:

$$\begin{aligned}
& > \text{solve}(\{\text{Capeq1}=0, \text{Capeq2}=0, \text{Capeq3}=0\}, \{B1, B2\}); \\
& \quad \{B1=0, B2=0\}
\end{aligned} \tag{7}$$

Now for the second Capparelli identity

Here, we have to take a sum of two expressions, as in equation (42).

The `beta` constants have some factors common.

Below, mp1 and mp2 denote those parts of beta1 and beta2 that are different

CapQ1, CapQ2 are the Q1 and Q2 constants corresponding to the matrix CapA.

```
> CapQ1:=3/4;
CapQ2:=2/(3^(2/3));
mp1:=(CapQ1^B1*CapQ2^B2);
mp2:=(CapQ1^B1p*CapQ2^B2p);
```

$$CapQ1 := \frac{3}{4}$$

$$CapQ2 := \frac{2}{3} 3^{1/3}$$

$$mp1 := \left(\frac{3}{4}\right)^{B1} \left(\frac{2}{3} 3^{1/3}\right)^{B2}$$

$$mp2 := \left(\frac{3}{4}\right)^{B1p} \left(\frac{2}{3} 3^{1/3}\right)^{B2p}$$

(8)

Now we calculate analogues of expressions appearing in (16) - (19) for this case.

We do not print out these expressions; they are quite big.

```
> Cap2expr1:=simplify(mp1*Capexpr1 + mp2*subs(B1=B1p,B2=B2p, C=C+
Cp, Capexpr1));
Cap2expr2:=simplify(mp1*Capexpr2 + mp2*subs(B1=B1p,B2=B2p, C=C+
Cp, Capexpr2));
Cap2expr3:=simplify(mp1*Capexpr3 + mp2*subs(B1=B1p,B2=B2p, C=C+
Cp, Capexpr3));
Cap2expr4:=simplify(mp1*Capexpr4 + mp2*subs(B1=B1p,B2=B2p, C=C+
Cp, Capexpr4));
```

Now we check if the sum-side for the second Capparelli identity gives all these expressions to be 0:

```
> Cap2C:=findC([-1, 1, -1, 0, -1, 0, -1, 0, -1, 1, -1, 0]);
subs(C=Cap2C,B1=1,B2=3,B1p=3,B2p=6,Cp=1,Cap2expr1);
subs(C=Cap2C,B1=1,B2=3,B1p=3,B2p=6,Cp=1,Cap2expr2);
subs(C=Cap2C,B1=1,B2=3,B1p=3,B2p=6,Cp=1,Cap2expr3);
subs(C=Cap2C,B1=1,B2=3,B1p=3,B2p=6,Cp=1,Cap2expr4);
```

$$Cap2C := \frac{5}{24}$$

0

0

0

0

(9)

Now we check numerically if there are other values of B\_1, B\_2, B\_1', B\_2', C' that satisfy the constraints.

```

> lb:=0;
ub:=6;
for b1 from lb to ub do:
for b2 from lb to ub do:
for b1p from b1 to ub do:
for b2p from b2 to ub do:
for cp from lb to ub do:

    cval:=solve(subs(B1=b1,B2=b2,B1p=b1p,B2p=b2p,Cp=cp,Cap2expr1)=
0);
    tempc2:=abs(subs(C=cval,B1=b1,B2=b2,B1p=b1p,B2p=b2p,Cp=cp,
Cap2expr2)):
    tempc3:=abs(subs(C=cval,B1=b1,B2=b2,B1p=b1p,B2p=b2p,Cp=cp,
Cap2expr3)):
    tempc4:=abs(subs(C=cval,B1=b1,B2=b2,B1p=b1p,B2p=b2p,Cp=cp,
Cap2expr4)):

    if (evalf(tempc2) < 0.001 and evalf(tempc3) < 0.001) and evalf
(tempc4) < 0.001 then:
        print("C=",cval," B1=",b1," B2=",b2," B1'=",b1p," B2'=",
b2p," C'=",cp):
        print("----"):
        fi:

od:
od:
od:
od:
od:

```

*lb := 0*

*ub := 6*

*"C=", - $\frac{1}{24}$ , " B1=", 0, " B2=", 0, " B1'=", 0, " B2'=", 0, " C'=", 0*

*----*

*"C=",  $\frac{5}{24}$ , " B1=", 1, " B2=", 0, " B1'=", 4, " B2'=", 6, " C'=", 1*

*----*

*"C=", - $\frac{1}{24}$ , " B1=", 1, " B2=", 0, " B1'=", 4, " B2'=", 6, " C'=", 2*

*----*

*"C=",  $\frac{5}{24}$ , " B1=", 1, " B2=", 3, " B1'=", 3, " B2'=", 6, " C'=", 1*

*----*

Now we look at the Mod-9 identities.  
 Since the analysis follows similarly, we skip the explanations.

```
> Mod9A:=Matrix(2,2,[2,3,3,6]);
Mod9At:=Mod9A+DiagonalMatrix([xi1,xi2]);
Mod9Atinv:=MatrixInverse(Mod9At);
```

$$\begin{aligned}
 \text{Mod9A} &:= \begin{bmatrix} 2 & 3 \\ 3 & 6 \end{bmatrix} \\
 \text{Mod9At} &:= \begin{bmatrix} 2 + \xi_1 & 3 \\ 3 & 6 + \xi_2 \end{bmatrix} \\
 \text{Mod9Atinv} &:= \begin{bmatrix} \frac{6 + \xi_2}{\xi_1 \xi_2 + 6 \xi_1 + 2 \xi_2 + 3} & -\frac{3}{\xi_1 \xi_2 + 6 \xi_1 + 2 \xi_2 + 3} \\ -\frac{3}{\xi_1 \xi_2 + 6 \xi_1 + 2 \xi_2 + 3} & \frac{2 + \xi_1}{\xi_1 \xi_2 + 6 \xi_1 + 2 \xi_2 + 3} \end{bmatrix}
 \end{aligned} \tag{11}$$

```
> Mod9Q1:=1-2*sin(Pi/18);
Mod9Q2:=(4*sin((1/18)*Pi)^2+4*sin((1/18)*Pi))^(1/3);

simplify(Mod9Q1^3 - 3*Mod9Q1^2 + 1);
simplify(Mod9Q2^9 - 6*Mod9Q2^6 + 3*Mod9Q2^3 + 1);
```

$$\begin{aligned}
 \text{Mod9Q1} &:= 1 - 2 \sin\left(\frac{1}{18} \pi\right) \\
 \text{Mod9Q2} &:= \left(4 \sin\left(\frac{1}{18} \pi\right)^2 + 4 \sin\left(\frac{1}{18} \pi\right)\right)^{1/3} \\
 &\quad \begin{matrix} 0 \\ 0 \end{matrix}
 \end{aligned} \tag{12}$$

We shall substitute actual values for xi's later:

```
> alias(zeta1=RootOf(x^3-3*x-1,x));
alias(zeta2=RootOf(x^3-9*x^2-54*x-27,x));
```

$$\begin{aligned}
 &\zeta_1, \zeta_2 \\
 &\zeta_1, \zeta_2
 \end{aligned} \tag{13}$$

```
> expargcutoff:=10;
expcutoff:=expargcutoff-2;

expargcutoff:=10
expcutoff:=8
```

```
> exptwovar:=serexp(ser(exparg(B1,xi1,T1,1,expargcutoff)+exparg(B2,
xi2,T2,3,expargcutoff),expcutoff,epsilon),expcutoff):
Mod9wanted:=ser(int2all(exptwovar,Mod9Atinv,20,T1,T2),
expargcutoff,epsilon):
> Mod9c1:=coeff(Mod9wanted,epsilon,2):
```

(14)

```

Mod9c2:=coeff(Mod9wanted,epsilon,4):
Mod9c3:=coeff(Mod9wanted,epsilon,6):
Mod9c4:=coeff(Mod9wanted,epsilon,8):
> Mod9g:=simplify(C+(2*zeta1+1)/24+(2*zeta2+3)/24);
Mod9expr1:=simplify(subs(xi1=zeta1,xi2=zeta2,Mod9c1-Mod9g));
Mod9expr2:=simplify(subs(xi1=zeta1,xi2=zeta2,Mod9c2-Mod9g*
Mod9c1+Mod9g^2/2));
Mod9expr3:=simplify(subs(xi1=zeta1,xi2=zeta2,Mod9c3-Mod9g*
Mod9c2+Mod9g^2/2*Mod9c1-Mod9g^3/6));

```

$$Mod9g := C + \frac{1}{12} \zeta_1 + \frac{1}{6} + \frac{1}{12} \zeta_2 \quad (15)$$

Now we check that the three Mod-9 identities satisfy the required constraints.

Identity 1:

```

> id1C:=findC([-1,0,-1,0,0,-1,0,-1,0]);
evalf(subs(C=id1C,B1=0,B2=0,Mod9expr1));
evalf(subs(C=id1C,B1=0,B2=0,Mod9expr2));
evalf(subs(C=id1C,B1=0,B2=0,Mod9expr3));

```

$$id1C := -\frac{1}{18}$$

$$\begin{aligned}
&4.1097240058012954533367242708530259123408456094164 \cdot 10^{-54} \\
&6.8403817185630757697220275314654830769375301306767 \cdot 10^{-58} \\
&6.0722094868465665674086652688149183815152250019421 \cdot 10^{-60}
\end{aligned} \quad (16)$$

Identity 2:

```

> id2C:=findC([0,-1,-1,0,0,-1,-1,0,0]);
evalf(subs(C=id2C,B1=1,B2=3,Mod9expr1));
evalf(subs(C=id2C,B1=1,B2=3,Mod9expr2));
evalf(subs(C=id2C,B1=1,B2=3,Mod9expr3));

```

$$id2C := \frac{5}{18}$$

0.

$$\begin{aligned}
&2.0521145155689227309166082594396449230812590392029 \cdot 10^{-57} \\
&0.
\end{aligned} \quad (17)$$

Identity 3:

```

> id3C:=findC([0,0,-1,-1,-1,-1,0,0,0]);
evalf(subs(C=id3C,B1=2,B2=3,Mod9expr1));
evalf(subs(C=id3C,B1=2,B2=3,Mod9expr2));
evalf(subs(C=id3C,B1=2,B2=3,Mod9expr3));

```

$$id3C := \frac{11}{18}$$

0.

0.

$$1.5180523717116416418521663172037295953788062504856 \cdot 10^{-58} \quad (18)$$

Now we proceed to the general search.

We do not print the output of the following commands, since they are quite big.

```
> Mod9cval:=solve (Mod9expr1=0,C) :  
Mod9eq1:=simplify (subs (C=Mod9cval,Mod9expr2)) :  
Mod9eq2:=simplify (subs (C=Mod9cval,Mod9expr3)) :  
> for b1 from -40 to 40 do:  
  for b2 from -40 to 40 do:  
    tempCval:=solve (subs (B1=b1,B2=b2,Mod9expr1)=0,C) :  
    Mod9eq2eval:=evalf (subs (B1=b1,B2=b2,Mod9eq1)) :  
    Mod9eq3eval:=evalf (subs (B1=b1,B2=b2,Mod9eq2)) :  
    if abs (Mod9eq2eval)<10^(-3) and abs (Mod9eq3eval)<10^(-3) then:  
      print ("C", identify (evalf (tempCval)), " B1", b1, " B2", b2) :  
  
    fi:  
  end:  
end:
```

"C",  $-\frac{1}{18}$ , " B1", 0, " B2", 0

"C",  $\frac{5}{18}$ , " B1", 1, " B2", 3

"C",  $\frac{11}{18}$ , " B1", 2, " B2", 3

(19)

Dilogarithm verification:

```
> evalf ((L(1) - L (Mod9Q1)) + (L(1)-L (Mod9Q2^3)) /3 - 2*Pi^2/27) ;  
  
-1.01 10-48
```

(20)
